# Supplementary material for: ZRG: A Dataset for Multimodal 3D Residential Rooftop Understanding
Source: arXiv:2304.13219 source file (2023-11-03)
Supplement: Supplementary file 1 [file appendix.tex]

\newpage
\appendix
\section{Implementation Details}
\label{sec:appendix-implementation-details}

For the following experiments described in Section~\ref{sec:experiments} we apply the following methods and training techniques throughout. We perform all experiments on a NVIDIA DGX server with 2 NVIDIA A100s consisting of 40GB each.

\subsection{Training Hyperparameters}
\label{sec:hparams}

We trained each baseline model with the common hyperparameters in Table \ref{tab:hyperparameters} below.

\input{tables/hparams}

\subsection{Data Augmentation}
\label{sec:augmentation}

During training we randomly augment the images and bounding boxes using the following methods:

\begin{itemize}
    \item Random Horizontal Flip with probability $p=0.5$
    \item Random Vertical Flip with probability $p=0.5$
    \item Random Rotation with degrees $d \in [0..90]$ and probability $p=0.25$
    \item Random Color Jitter with brightness, contrast, saturation, and hue factors of $\sigma=0.1$ and probability $p=0.25$
    \item Random Perspective Transform with distortion scale of $0.5$ and probability $p=0.1$
    \item Random Gaussian Blur with kernel size $k=3$ and standard deviation of $\sigma \in [0.1..1]$ and probability $p=0.1$
\end{itemize}
